# Supplementary material for: End-to-end correlated subgap states in hybrid nanowires
Source: arXiv:1908.05549 source file (2019-09-17)
Supplement: Supplementary file 1 [file supplement.pdf]

# Supplement to "End-to-end correlated subgap states in hybrid nanowires"


G. L. R. Anselmetti,[1] E. A. Martinez,[1] G. C. Ménard,[1] D. Puglia,[1] F. K. Malinowski,[1] J.S. Lee,[2] S. Choi,[2] M. Pendharkar,[3] C. J. Palmstrøm,[2,3,4] C. M. Marcus,[1] L. Casparis,[1,*] and A. P. Higginbotham[1,†]

[1]*Center for Quantum Devices, Niels Bohr Institute, University of Copenhagen, and Microsoft Quantum - Copenhagen, Universitetsparken 5, 2100 Copenhagen, Denmark*

[2]*California NanoSystems Institute, University of California, Santa Barbara, California 93106, USA*

[3]*Department of Electrical Engineering, University of California, Santa Barbara, California 93106, USA*

[4]*Materials Department, University of California, Santa Barbara, California 93106, USA*


## COMPARISON OF DIFFERENT BIASING CONFIGURATIONS

In the main text, the short-device and long-device datasets use different biasing configurations. Here we show that the two biasing methods give the same results by directly comparing them on the short device. Sweeping the right-bias voltage, $V_R$ while measuring $I_\mathrm{R}$ with $V_\mathrm{Al} = 0$ generates a map of subgap states [Fig. S1(a)], which is familiar from the main text. Sweeping the aluminum bias voltage, $V_\mathrm{Al}$ while measuring $I_\mathrm{R}$ with $V_\mathrm{R} = 0$ fixed reveals the same conductance features [Fig. S1(b)], but with the dependence on bias voltage inverted, as one would expect from the other side of the right junction being biased. Note that the $V_R$ and $V_\mathrm{Al}$ scans are interlaced so that switches and device instabilities effect the two plots symmetrically. The strong similarity between Fig. S1(a) and Fig. S1(b) explicitly demonstrates the equivalence of the two biasing configurations.

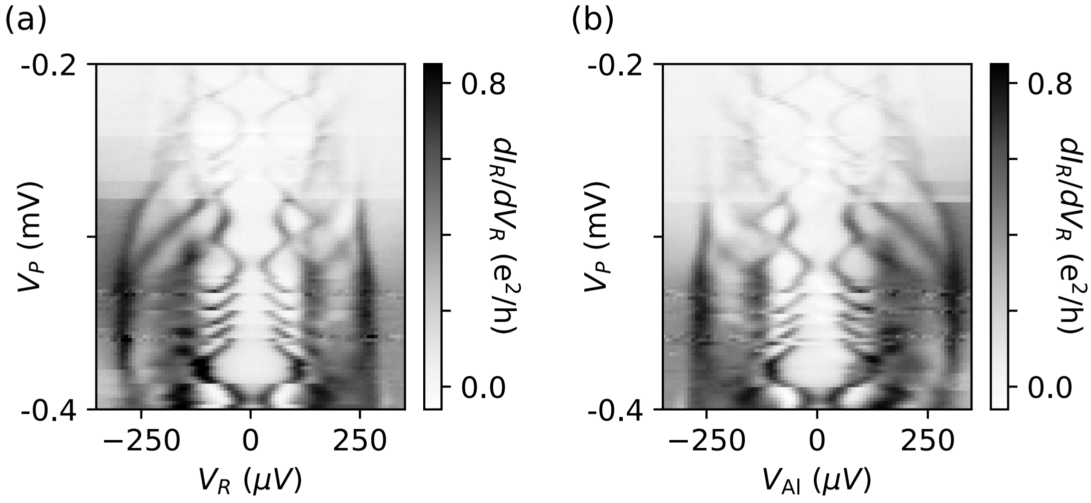


FIG. S1. (a) Right conductance, $dI_R/dV_R$, measured as a function of right bias, $V_R$ and plunger, $V_P$. In the main text, this biasing procedure was used for the short device. (b) Right conductance, $dI_R/dV_R$, measured as a function of aluminum bias, $V_\mathrm{Al}$, and plunger, $V_P$. In the main text, this biasing procedure was used for the long device.

## CORRELATOR ERROR ESTIMATES AND STATISTICAL INFORMATION

It is interesting to consider the error in the correlation metric, $\mathcal{C}$, that is computed in the main text Fig. 2. One method to estimate the uncertainty is to apply a numerical plunger-voltage shift, $\delta V_P$, to one dataset, compute the correlation metric $\mathcal{C}_{\delta V_P}$, and then find the standard deviation of $\sigma(\mathcal{C}_{\delta V_P})$ over a large ensemble of $\delta V_P$. Error bands in Fig. 3(c,d) are then given by $\overline{\mathcal{C}_{\delta V_P}} \pm \sigma(\mathcal{C}_{\delta V_P})$.

The computed error, $\sigma(\mathcal{C}_{\delta V_P})$, is compared with the data for the long-device correlator in Fig. S2. For large bias shifts, the correlator fluctuates but typically remains within the $1\sigma$ error bars, confirming that the error has been reasonably estimated. At zero bias shift, a $3\sigma$ peak in $\mathcal{C}$ is observed, with $4\sigma$ and $3\sigma$ satellite peaks, confirming that the corrrelations observed in the long device are statistically significant.

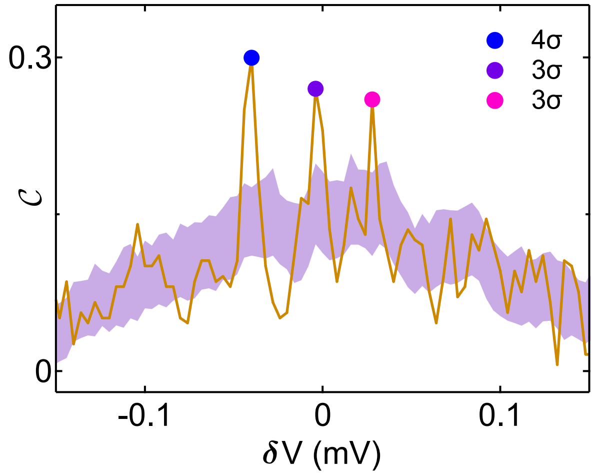


FIG. S2. Correlator, $\mathcal{C}$, for the long-device data set. Shaded region indicates $\pm 1\sigma$ error bars, estimated from plunger-shifted data. Colored circuls mark a $3\sigma$ central peak, with $4\sigma$ and $3\sigma$ satellite peaks.

When comparing the correlator between the short and long device it is useful to know that the properties of the two datasets are generally similar. The short-device data set has an average of 3.9 subgap peaks per bias scan, and the long-device data set has an average of 5.1 subgap peaks per bias scan. To evaluate the typical autocorrelation of the datasets, we have computed the self-mutual information, $SNMI$, of the conductances as a function of plunger shift, for instance $SNMI(\delta V_P) = NMI(g_R(V_P), g_R(V_P + \delta V_P))$. The self-mutual information decays as a function of plunger shift with a characteristic auto-correlation length. The extracted auto-correlation length is 4 mV for the short device, and 1.7 mV for the long device. The resolution on the datasets is one bias scan per 3.3 mV for the short device, and one bias scan per 0.5 mV for the long device.

## FULL DATASETS

For completeness, the full conductance datasets used in the main text are presented in Fig. S3. Most states in the short device can be identified on both sides, albeit with fluctuating weights [Fig. S3(a,b)]. The conductance associated low-lying stable bound state discussed in the main text has an anomalously large point-wise mutual information, $PMI$ [Fig. S3 (c)]. For the long device, most states are uncorrelated, but there is a small region of correlated features responsible for the correlator peak discussed in the main text [orange box Fig. S3(d,e)]. The conductance-$PMI$ for the long device is lower than the short device, with weak structure visible corresponding to the uncorrelated features [Fig. S3(f)].

## QUANTIFYING CONDUCTANCE CORRELATIONS WITH MUTUAL INFORMATION

In Fig. 4(a,b) of the main text we show the simultaneously measured left and right conductances as a scatter plot of $(g_L, g_R)$. Our goal is to quantify conductance correlations in this data. The conductances are correlated if they cannot be described by the product of two independent conductance distributions on the left and right sides. The statistical measure for how much the joint conductance distribution deviates from independence is given by the *mutual information* between the left and right conductances.

In the first place we seek to estimate the joint conductance probability distribution. For this we bin the measured conductance points to calculate a histogram and estimate a discrete probability distribution $p(g_L, g_R)$. A uniformly spaced grid is not suitable for our measured conductance data, since the density of points changes by orders of magnitude in different regions of the conductance space. Therefore we use the adaptive binning algorithm of [41], where the sample space is recursively divided in rectangular bins with an equal number of points. As a criterion for continuing the subdivision of a bin, we require there be a minimum number of points in the bin. For the analysis in Fig. 4 we stop subdividing bins with fewer than 80 points, which yields an average of 36 points per bin for the final subdivision. The end result of the algorithm is a grid of $M$ rectangles $A_i \times B_i$. The probability density $p(A_i \times B_i)$

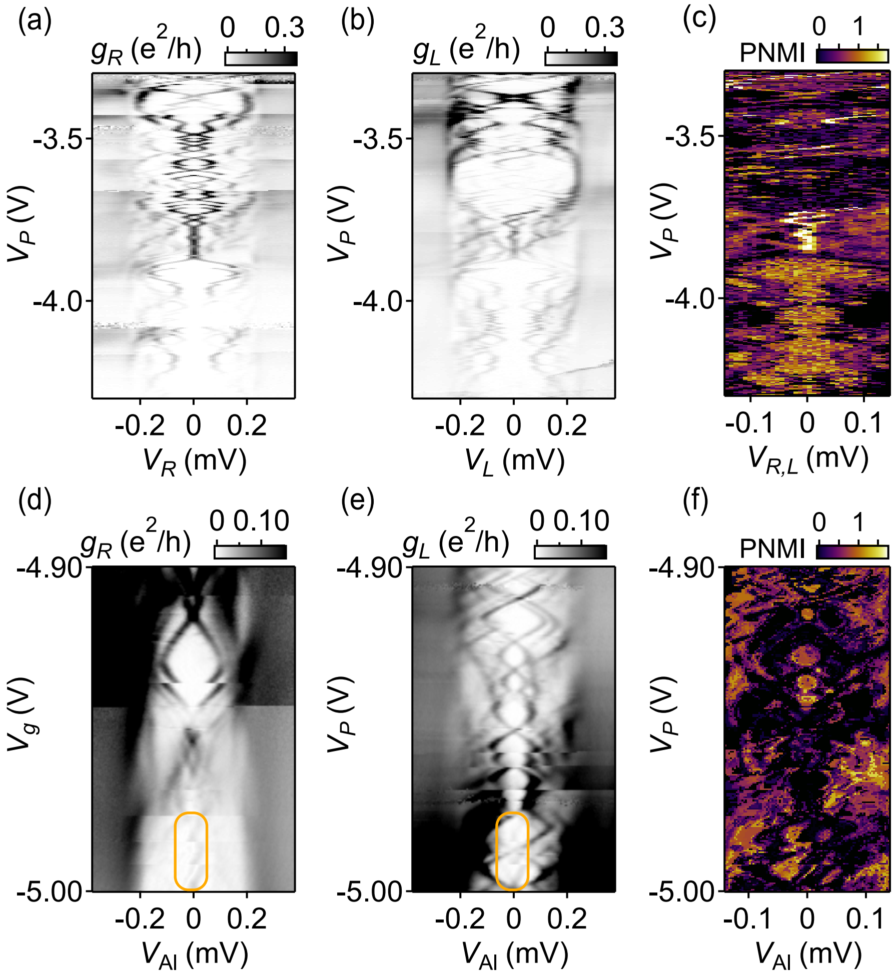


FIG. S3. (a) Short device right-conductance, $g_R$, measured as a function of gate, $V_P$ and bias, $V_R$. (b) Short device left-conductance, $g_L$, measured as a function of gate, $V_P$ and bias, $V_L$. (c) Short device conductance pointwise mutual information, $PMI$, mapped as a function of gate, $V_P$, and bias $V_{R,L}$ for subgap states. (d) Long device right-conductance, $g_R$, measured as a function of gate, $V_P$ and bias, $V_{\mathrm{Al}}$. Orange square indicates correlated region responsible for conductance peak in main text Fig. 3(d). (e) Long device left-conductance, $g_L$, measured as a function of gate, $V_P$ and bias, $V_{\mathrm{Al}}$. Orange squares indicates correlated region responsible for conductance peak in main text Fig. 3(d). (f) Long device conductance pointwise mutual information, $PMI$, mapped as a function of gate, $V_P$, and bias $V_{\mathrm{Al}}$ for subgap states.

in each bin $i$ is estimated as the number of samples in the bin divided by the total number of samples. The mutual information, MI, is then calculated as:

$$\mathrm{MI} = \sum_{i=1}^{M} p(A_i \times B_i) \log\left(\frac{p(A_i \times B_i)}{p(A_i \times \mathbb{R}) p(\mathbb{R} \times B_i)}\right), \tag{S1}$$

where $p(A_i \times \mathbb{R})$ is the probability density in the rectangle projected onto the left conductance axis, and $p(\mathbb{R} \times B_i)$ likewise projected onto the right conductance axis. The contribution of each bin in the sample space to the mutual information is known as the pointwise mutual information (PMI):

$$\mathrm{PMI} = \log\left(\frac{p(A_i \times B_i)}{p(A_i \times \mathbb{R}) p(\mathbb{R} \times B_i)}\right). \tag{S2}$$

The mutual information is the expected value of the pointwise mutual information over the entire distribution.

In the main text we quote the normalized mutual information, NMI, which lies in the range $[0, 1]$ and is given by

$$\mathrm{NMI} = \frac{\mathrm{MI}}{H}, \tag{S3}$$

where $H$ is the Shannon entropy of the joint probability distribution:

$$H = -\sum_{i=1}^{M} p(A_i \times B_i) \log p(A_i \times B_i). \tag{S4}$$

The main text also quotes the normalized pointwise mutual information, NPMI, given by

$$\text{NPMI} = \frac{\text{PMI}}{H}. \tag{S5}$$

Note that different normalization choices are possible, see e.g. [42].

The advantage of our selected method for calculating the mutual information is that the contribution of each bin can be easily assessed by visualizing the pointwise mutual information. This allows us to determine the relative contribution of the measured points to the total correlation, as shown by the maps of Fig. 4(e,f) in the main text. The drawback of the method, as with any method that relies on binning of the data, is the dependence of the calculated mutual information on the details of the binning. An alternative method for estimating the mutual information of the measured distribution is a non-parametric estimator, such as the one from [43]. This method relies only on the nearest-neighbor distances for estimating the mutual information. In Fig. S4 we compare the results obtained from the adaptive binning and the non-parametric algorithms, finding that they result in a similar numeric value. The calculations of the non-parametric estimator have been done using its implementation in the Python sklearn package[44].

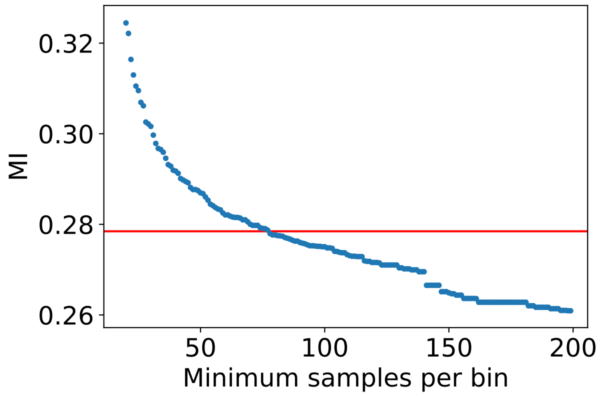


FIG. S4. Blue dots: mutual information (unnormalized) calculated with the adaptive binning method of [41] as a function of the minimum samples per bin cutoff for the subdivision algorithm. Red line: non-parametric estimate of the mutual information from [43].

* Equal contribution, lucas.casparis@microsoft.com
† Equal contribution, andrew.higginbotham@ist.ac.at
